# Supplementary material for: Persistent Weak Interferer Detection in WiFi Networks: A Deep Learning Based Approach
Source: arXiv:2205.11360 source file (2022-05-23)
Supplement: Supplementary file 3 [file C.tex]

% Investigation of MSP performance

The MSP model trained without OE is found degrades in performance over lower SIR ranges for QPSK and 16-QAM subcarrier modulation types. \figref*{fig:msp_comparison} shows the performance of the the MSP model (without OE) with a modification such that when test sample subcarrier modulation types are misclassified, their maximum softmax probabilities are set to 0.25, which is the maximum softmax probability for a uniform distribution. The purpose of showing the results of this ``Modified" approach is to identify the cause of performance degradation in low SIR ranges.

\figref*{fig:msp_comparison} shows that the ``Modified" anomaly detection method for MSP mitigates AUROC degradation for higher SIR bins. This increase in anomaly detection performance shows that performance degradation occurs only when samples are misclassified with high confidence, since reducing the confidence only for misclassified samples improves AUROC.

\newpage
\begin{figure}[ht!]
\begin{center}
    \includegraphics[scale=0.5]{plots/Results/msp_comparison.png}
    \caption[]{MSP Model performance with and without "Modified" approach.}
    \label{fig:msp_comparison}
\end{center}
\end{figure}
